# Supplementary material for: SU(4) lattice gauge theory with decuplet fermions: Schr\"odinger functional analysis
Source: arXiv:1202.2675 ancillary file (2012-02-13)
Supplement: Supplementary file 1 [file AppendixA.pdf]

Attachment to

T. DeGrand, Y. Shamir, and B. Svetitsky, *SU(4) lattice gauge theory with decuplet fermions...*, Appendix A

## Coefficients for U(n) projection (and its derivative): U(3) and U(4)

Set  $n = 3$  or 4 for  $SU(n)$

In[1]:= **n = 4;**

$r_i = \sqrt{g_i}$  -- use instead of  $g_i$  everywhere

In[2]:= **SG = Table[r<sub>i</sub>, {i, 0, n - 1}]**

Out[2]= {r<sub>0</sub>, r<sub>1</sub>, r<sub>2</sub>, r<sub>3</sub>}

set of symmetric polynomials -- 3 or 4 of them

In[3]:= **SP = If[n == 3, {u, v, w}, {u, v, w, x}]**

Out[3]= {u, v, w, x}

Vandermonde matrix  $\partial c_i / \partial g_j$

In[4]:= **VM = Table[r<sub>i</sub>^(2 j), {j, 0, n - 1}, {i, 0, n - 1}]; MatrixForm[VM]**

Out[4]//MatrixForm =

$$\begin{pmatrix} 1 & 1 & 1 & 1 \\ r_0^2 & r_1^2 & r_2^2 & r_3^2 \\ r_0^4 & r_1^4 & r_2^4 & r_3^4 \\ r_0^6 & r_1^6 & r_2^6 & r_3^6 \end{pmatrix}$$

Invert it.

In[5]:= **VMI = Together[Inverse[VM]]; MatrixForm[VMI]**

Out[5]//MatrixForm =

$$\begin{pmatrix} \frac{r_1^2 r_2^2 r_3^2}{(-r_0^2+r_1^2)(-r_0^2+r_2^2)(-r_0^2+r_3^2)} & \frac{-r_1^2 r_2^2-r_1^2 r_3^2-r_2^2 r_3^2}{(-r_0^2+r_1^2)(-r_0^2+r_2^2)(-r_0^2+r_3^2)} & \frac{r_1^2+r_2^2+r_3^2}{(-r_0^2+r_1^2)(-r_0^2+r_2^2)(-r_0^2+r_3^2)} & -\frac{1}{(-r_0^2+r_1^2)(-r_0^2+r_2^2)(-r_0^2+r_3^2)} \\ \frac{r_0^2 r_2^2 r_3^2}{(r_0^2-r_1^2)(-r_1^2+r_2^2)(-r_1^2+r_3^2)} & \frac{-r_0^2 r_2^2-r_0^2 r_3^2-r_2^2 r_3^2}{(r_0^2-r_1^2)(-r_1^2+r_2^2)(-r_1^2+r_3^2)} & \frac{r_0^2+r_2^2+r_3^2}{(r_0^2-r_1^2)(-r_1^2+r_2^2)(-r_1^2+r_3^2)} & -\frac{1}{(r_0^2-r_1^2)(-r_1^2+r_2^2)(-r_1^2+r_3^2)} \\ \frac{r_0^2 r_1^2 r_3^2}{(r_0^2-r_2^2)(r_1^2-r_2^2)(-r_2^2+r_3^2)} & \frac{-r_0^2 r_1^2-r_0^2 r_3^2-r_1^2 r_3^2}{(r_0^2-r_2^2)(r_1^2-r_2^2)(-r_2^2+r_3^2)} & \frac{r_0^2+r_1^2+r_3^2}{(r_0^2-r_2^2)(r_1^2-r_2^2)(-r_2^2+r_3^2)} & -\frac{1}{(r_0^2-r_2^2)(r_1^2-r_2^2)(-r_2^2+r_3^2)} \\ \frac{r_0^2 r_1^2 r_2^2}{(r_0^2-r_3^2)(r_1^2-r_3^2)(r_2^2-r_3^2)} & \frac{-r_0^2 r_1^2-r_0^2 r_2^2-r_1^2 r_2^2}{(r_0^2-r_3^2)(r_1^2-r_3^2)(r_2^2-r_3^2)} & \frac{r_0^2+r_1^2+r_2^2}{(r_0^2-r_3^2)(r_1^2-r_3^2)(r_2^2-r_3^2)} & -\frac{1}{(r_0^2-r_3^2)(r_1^2-r_3^2)(r_2^2-r_3^2)} \end{pmatrix}$$

Matrix for Eq. (A4)

In[6]:= **M = Transpose[VM]; MatrixForm[M]**

Out[6]//MatrixForm =

$$\begin{pmatrix} 1 & r_0^2 & r_0^4 & r_0^6 \\ 1 & r_1^2 & r_1^4 & r_1^6 \\ 1 & r_2^2 & r_2^4 & r_2^6 \\ 1 & r_3^2 & r_3^4 & r_3^6 \end{pmatrix}$$

RHS of Eq. (A4)

```
In[7]:= W = Table[1 / ri, {i, 0, n - 1}]
```

```
Out[7]= { 1 / r0, 1 / r1, 1 / r2, 1 / r3 }
```

$f_i$ , from solving Eq. (A4)

```
In[8]:= F = Together[Inverse[M].W];
```

Write  $f_i$  in terms of the symmetric polynomials. (Use `CForm[ ]` to get output that is usable in a C program.)

```
In[9]:= For[i = 1, i ≤ n, i++,
  NUM[i] = Simplify[SymmetricReduction[Numerator[Together[F[[i]]]], SG, SP]];
  Print[NUM[i][[1]]]
]
```

```
-w3 - u2 w x + v w x + u (v w2 - v2 x + x2)
```

```
2 u2 v w - u (v3 + 2 w2) - u3 x + w (v2 + x)
```

```
u3 v - u2 w + 2 v w + u (-2 v2 + x)
```

```
-u v + w
```

```
In[10]:= DEN = Simplify[SymmetricReduction[Denominator[Together[F[[1]]]], SG, SP][[1]]]
```

```
Out[10]= -x (-u v w + w2 + u2 x)
```

(Check that the denominator is really a common denominator!)

Now for the chain rule:  $\partial f_i / \partial g_j$

```
In[11]:= DRV = Table[D[F[[i]], rj] / (2 rj), {i, 1, n}, {j, 0, n - 1}];
```

Multiply by  $\partial g_j / \partial c_k$ , giving the  $b$  coefficients [Eq.(A15)]

```
In[12]:= B = Together[DRV.VMI];
```

Print in terms of symmetric polynomials.

```
In[13]:= For[i = 1, i ≤ n, i++,
  For[j = i, j ≤ n, j++,
    NUMB[i, j] = Simplify[SymmetricReduction[Numerator[Together[B[[i]][[j]]]], SG, SP]];
    Print[NUMB[i, j][[1]]]
  ]
]
```

```
u7 x5 + u6 w x3 (w2 - 8 v x) + u5 x2 (-3 v w4 + 16 v2 w2 x - 4 v3 x2 + 5 w2 x2 + 4 v x3) +
w3 (w6 - 3 v w4 x - w2 x3 + v (v2 - 2 x) x3) - 3 u w2 (v w6 - w4 x2 + v4 x3 + x5 - 3 v2 x (w4 + x3)) +
u4 w x (-12 v3 w2 x + 3 w4 x + 3 v4 x2 - 23 v w2 x2 - 4 x4 + v2 (3 w4 + 4 x3)) +
u2 w (3 w6 x + 3 v5 x3 - 4 w2 x4 + 9 v x2 (-2 w4 + x3) + 3 v2 (w6 + 2 w2 x3) - 3 v3 (3 w4 x + 4 x4)) +
u3 (-v6 x3 + 7 w4 x3 + x6 - v3 (w6 + 8 w2 x3) + v4 (3 w4 x + 5 x4) + v (-6 w6 x + 4 w2 x4) + 3 v2 (9 w4 x2 - 2 x5))
```

$$\begin{aligned}
& u^7 x^3 (2 w^2 - 3 v x) - u^6 w x^2 (6 v w^2 - 10 v^2 x + x^2) - w^3 (-v^3 w^2 x + 2 w^4 x - v^4 x^2 + x^4 + v^2 (w^4 + x^3)) + \\
& u^5 x (-6 v^3 w^2 x + 6 w^4 x - 5 v^4 x^2 - 10 v w^2 x^2 + 2 v^2 (3 w^4 + x^3)) - \\
& u^2 w (-3 v^5 w^2 x + 3 v^2 w^4 x - 3 v^6 x^2 - 12 v^3 w^2 x^2 + 3 x^2 (w^4 - x^3) + 3 v^4 (w^4 + 3 x^3) + v (6 w^6 + 5 w^2 x^3)) - \\
& u^4 w (v^4 w^2 x - 6 v^5 x^2 - 12 v^2 w^2 x^2 + w^2 x^3 + 2 v^3 (w^4 - x^3) + 4 v (3 w^4 x - x^4)) + \\
& u w^2 (2 w^6 - 3 v^4 w^2 x - 3 v^5 x^2 - 3 v^2 w^2 x^2 + 3 v^3 (w^4 + 2 x^3) + v (4 w^4 x + 3 x^4)) - u^3 (v^6 w^2 x - 6 w^6 x + v^7 x^2 + \\
& 15 v^4 w^2 x^2 + 5 w^2 x^4 - v^5 (w^4 + 4 x^3) - 2 v^2 (3 w^6 + 4 w^2 x^3) + v^3 (-2 w^4 x + 2 x^4) + v (3 w^4 x^2 + 2 x^5)) \\
& u^8 w x^3 - u^7 x^2 (3 v w^2 - 4 v^2 x + x^2) + u^6 w x (3 v^2 w^2 - 4 v^3 x + 3 w^2 x - 7 v x^2) - \\
& w^3 (2 v w^4 - 2 v^2 w^2 x - 2 v^3 x^2 + w^2 x^2 + 3 v x^3) + u w^2 (-6 v^3 w^2 x - 6 v^4 x^2 + v w^2 x^2 - 3 x^4 + 3 v^2 (2 w^4 + 5 x^3)) + \\
& u^4 w (-9 v^3 w^2 x + 5 v^4 x^2 - 12 v w^2 x^2 + 3 x (w^4 - 2 x^3) + v^2 (3 w^4 + 16 x^3)) + \\
& u^3 (-2 v^5 w^2 x - 2 v^6 x^2 - 14 v^3 w^2 x^2 + x^2 (w^4 + x^3) + v^4 (2 w^4 + 9 x^3) - v (3 w^6 + 2 w^2 x^3) + 3 v^2 (5 w^4 x - 3 x^4)) + \\
& u^5 (v^4 w^2 x + v^5 x^2 + 15 v^2 w^2 x^2 + w^2 x^3 - v^3 (w^4 + 12 x^3) + v (-6 w^4 x + 8 x^4)) + \\
& u^2 w (w^6 + 6 v^4 w^2 x + 6 v^5 x^2 + 8 v^2 w^2 x^2 - 2 w^2 x^3 - 3 v^3 (2 w^4 + 7 x^3) + v (-7 w^4 x + 12 x^4)) \\
& - u^6 w x^3 + u^5 x^2 (3 v w^2 - 4 v^2 x + x^2) + u^4 w x (-3 v^2 w^2 + 4 v^3 x - 3 w^2 x + 5 v x^2) - w^3 (w^4 - v w^2 x + x^2 (-v^2 + x)) - \\
& u w^2 (3 v^2 w^2 x + 3 v^3 x^2 + w^2 x^2 - 3 v (w^4 + 2 x^3)) + 3 u^2 w (v^3 w^2 x - w^4 x + v^4 x^2 + 2 v w^2 x^2 + x^4 - v^2 (w^4 + 3 x^3)) - \\
& u^3 (v^4 w^2 x + v^5 x^2 + 9 v^2 w^2 x^2 + w^2 x^3 - v^3 (w^4 + 4 x^3) + v (-6 w^4 x + 3 x^4)) \\
& 3 u^8 w x^3 - 3 u^7 x^2 (4 v w^2 + v^2 x + x^2) + \\
& u^6 w x (12 v^2 w^2 + 16 v^3 x + 12 w^2 x + 15 v x^2) + w^3 (v^4 w^2 + v^5 x + 4 v^2 w^2 x + 2 w^2 x^2 - v x^3) - \\
& u w^2 (3 v^5 w^2 + 3 v^6 x + 16 v^3 w^2 x + 8 w^4 x - 3 v^4 x^2 + 6 v w^2 x^2 - 3 x^4 + v^2 (4 w^4 - 6 x^3)) + \\
& u^2 w (3 v^6 w^2 + 4 w^6 + 3 v^7 x + 27 v^4 w^2 x + 28 v w^4 x - 6 v^5 x^2 + 8 v^2 w^2 x^2 - 3 w^2 x^3 + 6 v^3 (2 w^4 - x^3)) - \\
& u^5 (16 v^4 w^2 x + 24 v w^4 x + 5 v^5 x^2 + 36 v^2 w^2 x^2 + 17 w^2 x^3 + 4 v^3 (w^4 + x^3)) + \\
& u^4 w (4 v^5 w^2 + 7 v^6 x + 44 v^3 w^2 x + 9 v^4 x^2 + 36 v w^2 x^2 + 4 v^2 (3 w^4 + 2 x^3) + 4 (3 w^4 x + x^4)) - \\
& u^3 (v^7 w^2 + 12 v w^6 + v^8 x + 22 v^5 w^2 x - 3 v^6 x^2 + 8 v^3 w^2 x^2 + 16 w^4 x^2 + x^5 + v^4 (12 w^4 - x^3) + 2 v^2 (24 w^4 x + x^4)) \\
& - 6 u^8 v w x^2 + u^9 x^3 + 2 u^7 x (3 v^2 w^2 + 2 v^3 x + 3 w^2 x) + \\
& w^3 (2 v^3 w^2 + 2 v^4 x + 4 v w^2 x - v^2 x^2 - x^3) - u^6 w (2 v^3 w^2 + 5 v^4 x + 12 v w^2 x - 6 v^2 x^2 + 5 x^3) + \\
& u w^2 (-6 v^4 w^2 - 4 v w^4 - 6 v^5 x - 16 v^2 w^2 x + 9 v^3 x^2 + 2 w^2 x^2 + 6 v x^3) + \\
& u^4 w (v^4 w^2 - 6 v w^4 + 7 v^5 x + 9 v^2 w^2 x + 16 v^3 x^2 - w^2 x^2 + 10 v x^3) + \\
& u^2 w (6 v^5 w^2 + 6 v^6 x + 29 v^3 w^2 x - 2 w^4 x - 15 v^4 x^2 - 4 v w^2 x^2 + 3 x^4 + v^2 (11 w^4 - 3 x^3)) + \\
& u^5 (v^5 w^2 + v^6 x + 2 v^3 w^2 x - 11 v^4 x^2 - 9 v w^2 x^2 + v^2 (6 w^4 - 2 x^3) + 2 x (3 w^4 + x^3)) - \\
& u^3 (2 v^6 w^2 - 2 w^6 + 2 v^7 x + 25 v^4 w^2 x - 7 v^5 x^2 + 3 v^2 w^2 x^2 + 5 w^2 x^3 + v^3 (9 w^4 + 2 x^3) + v (4 w^4 x + 3 x^4)) \\
& v^2 w^5 + v^3 w^3 x + 2 w^5 x + 6 u^6 v w x^2 - u^7 x^3 - 2 u^5 x (3 v^2 w^2 + 2 v^3 x + 3 w^2 x + v x^2) - \\
& u w^2 (3 v^3 w^2 + 2 w^4 + 3 v^4 x + 8 v w^2 x - 3 v^2 x^2 - 3 x^3) + u^4 w (2 v^3 w^2 + 5 v^4 x + 12 v w^2 x + 6 v^2 x^2 + 4 x^3) + \\
& u^2 w (3 v^4 w^2 + 6 v w^4 + 3 v^5 x + 15 v^2 w^2 x - 6 v^3 x^2 + w^2 x^2 - 3 v x^3) - \\
& u^3 (v^5 w^2 + 6 v^2 w^4 + v^6 x + 14 v^3 w^2 x + 6 w^4 x - 3 v^4 x^2 + 3 v w^2 x^2 + x^4) \\
& - 3 u^9 v x^2 + 3 u^8 w x (v^2 + x) + 4 v w^3 (v w^2 + v^2 x - x^2) + 3 u^6 w (v^2 w^2 - 3 v^3 x + w^2 x - 6 v x^2) - \\
& 3 u w^2 (4 v^3 w^2 + 4 v^4 x - 8 v^2 x^2 + x^3) - u^7 (v^3 w^2 + v^4 x + 6 v w^2 x - 15 v^2 x^2 + 3 x^3) + \\
& u^2 w (12 v^4 w^2 - 4 v w^4 + 12 v^5 x + 8 v^2 w^2 x - 36 v^3 x^2 + 2 w^2 x^2 + 15 v x^3) + \\
& u^4 (-12 v^3 w^3 + w^5 - 11 v w^3 x + 42 v^2 w x^2 - 7 w x^3) + \\
& u^3 (-4 v^5 w^2 - 4 v^6 x - 12 v^3 w^2 x + 16 v^4 x^2 - 18 v w^2 x^2 + x^4 + v^2 (12 w^4 - 13 x^3)) + \\
& u^5 (4 v^4 w^2 + 4 v^5 x + 21 v^2 w^2 x - 26 v^3 x^2 + 3 w^2 x^2 - 3 v (w^4 - 4 x^3))
\end{aligned}$$

$$\begin{aligned}
& 3 u^7 v x^2 - 3 u^6 w x (v^2 + x) - 3 u v w^2 (2 v w^2 + 2 v^2 x - 3 x^2) + \\
& w^3 (2 v w^2 + 2 v^2 x - x^2) - 3 u^4 w (v^2 w^2 - v^3 x + w^2 x - 4 v x^2) + \\
& u^5 (v^3 w^2 + v^4 x + 6 v w^2 x - 9 v^2 x^2 + 2 x^3) + u^2 w (6 v^3 w^2 - w^4 + 6 v^4 x + 5 v w^2 x - 15 v^2 x^2 + 3 x^3) - \\
& u^3 (2 v^4 w^2 - 3 v w^4 + 2 v^5 x + 9 v^2 w^2 x - 7 v^3 x^2 + 3 w^2 x^2 + 4 v x^3) \\
& w^5 + v w^3 x - 3 u^5 v x^2 + 3 u^4 w x (v^2 + x) - 3 u w^2 (v w^2 + v^2 x - x^2) + \\
& 3 u^2 w (v^2 w^2 + v^3 x + w^2 x - 2 v x^2) - u^3 (v^3 w^2 + v^4 x + 6 v w^2 x - 3 v^2 x^2 + x^3)
\end{aligned}$$

In[14]:= **DENB = SymmetricReduction[Denominator[Together[B[[1]][[1]]]], SG, SP][[1]]**

Out[14]=  $2 u^3 v^3 w^3 x^3 - 6 u^2 v^2 w^4 x^3 + 6 u v w^5 x^3 - 2 w^6 x^3 -$   
 $6 u^4 v^2 w^2 x^4 + 12 u^3 v w^3 x^4 - 6 u^2 w^4 x^4 + 6 u^5 v w x^5 - 6 u^4 w^2 x^5 - 2 u^6 x^6$

In[15]:= **Factor[DENB]**

Out[15]=  $-2 x^3 (-u v w + w^2 + u^2 x)^3$
